# Supplementary material for: Exciton radiative lifetimes in hexagonal diamond Ge and Si$_x$Ge$_{1-x}$ alloys
Source: arXiv:2512.15559 ancillary file (2026-04-14)
Supplement: Supplementary file 1 [file supplemental_material.pdf]

# Supplemental Material

## Exciton radiative lifetimes in hexagonal diamond Ge and $\text{Si}_x\text{Ge}_{1-x}$ alloys

Michele Re Fiorentin<sup>1,\*</sup>, Michele Amato<sup>2</sup> and Maurizia Palummo<sup>3</sup>

<sup>1</sup>*Department of Applied Science and Technology, Politecnico di Torino  
corso Duca degli Abruzzi 24, 10129 Torino, Italy*

<sup>2</sup>*Université Paris-Saclay, CNRS, Laboratoire de Physique des Solides, 91405 Orsay, France*

<sup>3</sup>*Dipartimento di Fisica and INFN, Università di Roma “Tor Vergata”,  
via della Ricerca Scientifica 1, 00133, Roma, Italy*

### S1 Optimized structures

The optimized geometries are shown in Fig. S1.

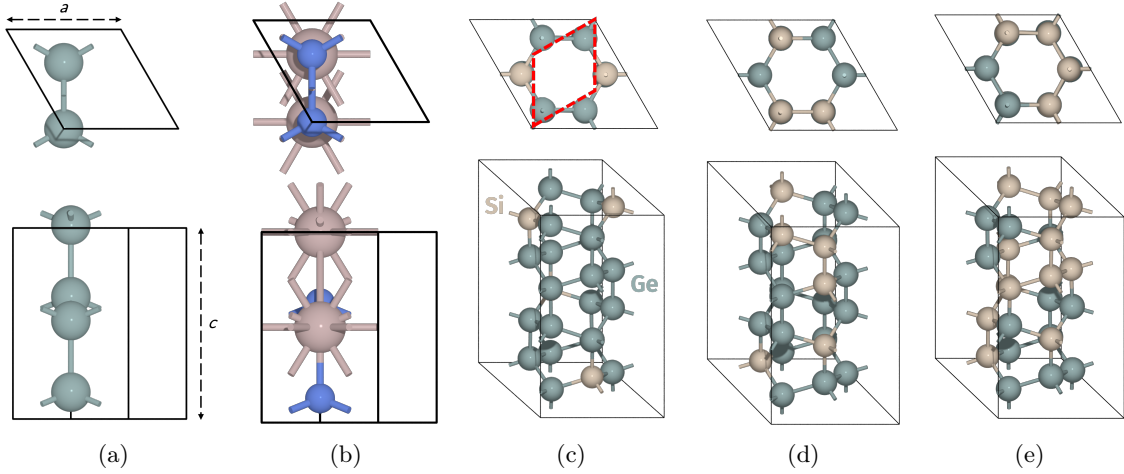

Figure S1: Optimized geometries of 2H-Ge in panel (a), GaN in (b) and the special quasi-random structure realizations of the  $\text{Si}_x\text{Ge}_{1-x}$  alloys:  $x = 1/6$  in (c),  $x = 1/4$  in (d) and  $x = 1/2$  in (e).

The corresponding lattice parameters are reported in Table S1

|                                      | $a$ (Å) | $c$ (Å) |
|--------------------------------------|---------|---------|
| 2H-Ge                                | 4.05    | 6.68    |
| 2H-Ge $\epsilon_z = 2\%$             | 4.05    | 6.81    |
| GaN                                  | 3.22    | 5.24    |
| 2H- $\text{Si}_{1/6}\text{Ge}_{5/6}$ | 6.94    | 13.23   |
| 2H- $\text{Si}_{1/4}\text{Ge}_{3/4}$ | 6.90    | 13.16   |
| 2H- $\text{Si}_{1/2}\text{Ge}_{1/2}$ | 6.80    | 12.97   |

Table S1: Lattice parameters of the studied systems.

The fractional coordinates of the Si and Ge atoms in the  $\text{Si}_x\text{Ge}_{1-x}$  alloys are reported below.

---

\*michele.refiorentin@polito.it

|                                            |    |              |              |              |
|--------------------------------------------|----|--------------|--------------|--------------|
| <b>2H-Si<sub>1/6</sub>Ge<sub>5/6</sub></b> | Ge | 0.1672820886 | 0.1735087036 | 0.9057969850 |
|                                            | Ge | 0.1666257370 | 0.5007488543 | 0.1567261717 |
|                                            | Ge | 0.1735600808 | 0.1674302375 | 0.0946532302 |
|                                            | Ge | 0.1730429604 | 0.5068736037 | 0.3444958813 |
|                                            | Ge | 0.1674830413 | 0.1671681887 | 0.4059937123 |
|                                            | Ge | 0.1667249536 | 0.5009067825 | 0.6602037014 |
|                                            | Ge | 0.1671338019 | 0.1675579806 | 0.5944206506 |
|                                            | Ge | 0.8326193668 | 0.8325588800 | 0.1560230145 |
|                                            | Ge | 0.8272968175 | 0.4931141880 | 0.0908319206 |
|                                            | Ge | 0.8264543366 | 0.8328408253 | 0.3446773153 |
|                                            | Ge | 0.8330041788 | 0.4991781510 | 0.4061579033 |
|                                            | Ge | 0.8324173887 | 0.8325903969 | 0.6563722925 |
|                                            | Ge | 0.8337359437 | 0.4995110744 | 0.5936998784 |
|                                            | Ge | 0.8329655138 | 0.8264560413 | 0.8450049165 |
|                                            | Ge | 0.4930380884 | 0.8272447190 | 0.9059719384 |
|                                            | Ge | 0.4992710729 | 0.8394161060 | 0.0939325874 |
|                                            | Ge | 0.5004955531 | 0.1602751040 | 0.3408412369 |
|                                            | Ge | 0.5007274108 | 0.1664958049 | 0.6565506973 |
|                                            | Ge | 0.4990703083 | 0.8329239583 | 0.5906065102 |
|                                            | Ge | 0.5069667236 | 0.1729947250 | 0.8443113248 |
|                                            | Si | 0.1600474188 | 0.5005078475 | 0.8451196536 |
|                                            | Si | 0.8396187417 | 0.4991939632 | 0.9056975480 |
|                                            | Si | 0.5009149118 | 0.1667491532 | 0.1559508208 |
|                                            | Si | 0.4995035610 | 0.8337547110 | 0.4059601089 |

|                                     |    |              |              |              |
|-------------------------------------|----|--------------|--------------|--------------|
| $2\text{H-Si}_{1/4}\text{Ge}_{3/4}$ | Si | 0.1751210700 | 0.1675662453 | 0.9053754995 |
|                                     | Si | 0.1678575609 | 0.5000403817 | 0.1542063830 |
|                                     | Si | 0.4989034261 | 0.8407811425 | 0.9053727634 |
|                                     | Si | 0.4994214446 | 0.1660943772 | 0.3425526381 |
|                                     | Si | 0.4988323172 | 0.1655042625 | 0.6622222771 |
|                                     | Si | 0.4927848257 | 0.1594630007 | 0.8430678317 |
|                                     | Ge | 0.1695251886 | 0.1734634023 | 0.0904514179 |
|                                     | Ge | 0.1672699378 | 0.4999924079 | 0.3396786350 |
|                                     | Ge | 0.1749164009 | 0.1677620840 | 0.4056735895 |
|                                     | Ge | 0.1675790286 | 0.4999876030 | 0.6572308478 |
|                                     | Ge | 0.1754415593 | 0.1672031989 | 0.5948785123 |
|                                     | Ge | 0.1736956098 | 0.5001518859 | 0.8458621082 |
|                                     | Ge | 0.8260402865 | 0.4917836692 | 0.9054906380 |
|                                     | Ge | 0.8333862261 | 0.8344403062 | 0.1543192284 |
|                                     | Ge | 0.8375081659 | 0.4973962327 | 0.0944081215 |
|                                     | Ge | 0.8333171976 | 0.8339100157 | 0.3436573290 |
|                                     | Ge | 0.8261684287 | 0.4917422006 | 0.4055868932 |
|                                     | Ge | 0.8333157735 | 0.8342475693 | 0.6571760565 |
|                                     | Ge | 0.8249770193 | 0.4910672445 | 0.5958622523 |
|                                     | Ge | 0.8334802029 | 0.8404247523 | 0.8468084199 |
|                                     | Ge | 0.4989277623 | 0.1655831256 | 0.1591152565 |
|                                     | Ge | 0.4932641494 | 0.8293804507 | 0.0904510027 |
|                                     | Ge | 0.4988836942 | 0.8404777656 | 0.4056738872 |
|                                     | Ge | 0.4993827243 | 0.8415366759 | 0.5948784115 |

|                                     |    |              |              |              |
|-------------------------------------|----|--------------|--------------|--------------|
| $2\text{H-Si}_{1/2}\text{Ge}_{1/2}$ | Ge | 0.1681615283 | 0.1613280754 | 0.9035700832 |
|                                     | Ge | 0.1685266399 | 0.1736639014 | 0.0950859626 |
|                                     | Ge | 0.1745535696 | 0.1738803254 | 0.4085477049 |
|                                     | Ge | 0.1675962312 | 0.5018037584 | 0.6529525012 |
|                                     | Ge | 0.1671503705 | 0.5073579388 | 0.8432130095 |
|                                     | Ge | 0.8311857411 | 0.8322278523 | 0.1565059659 |
|                                     | Ge | 0.8384056703 | 0.4981914644 | 0.0910649192 |
|                                     | Ge | 0.8260087848 | 0.8327163522 | 0.3470125492 |
|                                     | Ge | 0.8329253838 | 0.4921925765 | 0.4085346260 |
|                                     | Ge | 0.8312771267 | 0.8322768474 | 0.6558470984 |
|                                     | Ge | 0.5012489580 | 0.1655975314 | 0.1604595843 |
|                                     | Ge | 0.4932369317 | 0.8284610919 | 0.0899400515 |
|                                     | Si | 0.1679108163 | 0.5025750067 | 0.1595068925 |
|                                     | Si | 0.1734594633 | 0.5075229726 | 0.3431814781 |
|                                     | Si | 0.1745534091 | 0.1671769329 | 0.5959581060 |
|                                     | Si | 0.8262081929 | 0.4983167683 | 0.9033421212 |
|                                     | Si | 0.8260754531 | 0.4920858179 | 0.5949560866 |
|                                     | Si | 0.8256981383 | 0.8263415280 | 0.8443710895 |
|                                     | Si | 0.5055468424 | 0.8403460693 | 0.9032865879 |
|                                     | Si | 0.5004459010 | 0.1597598512 | 0.3460682021 |
|                                     | Si | 0.4923835760 | 0.8338066672 | 0.4085805762 |
|                                     | Si | 0.5010313784 | 0.1655571639 | 0.6566461128 |
|                                     | Si | 0.4993261995 | 0.8405852298 | 0.5910601823 |
|                                     | Si | 0.5070836939 | 0.1662282768 | 0.8403085088 |

## S2 Computational details

In Fig. S2 we report the change in the electronic bandgap of 2H-Ge with varying  $J$  parameter. The value obtained by the HSE06 calculation, marked by the dashed horizontal line, is matched for  $J \simeq 23$  eV.

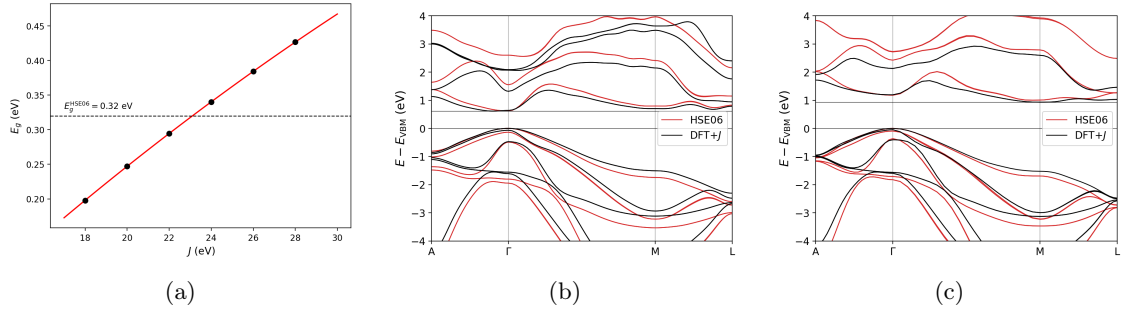

Figure S2: (a) Variation of the bandgap of pristine 2H-Ge at different  $J$  values. (b) Comparison of the bandstructures computed with the HSE06 functional (red lines) and with DFT+ $J$  (black lines) with  $J = 40$  eV for a 2H-Si<sub>1/4</sub>Ge<sub>3/4</sub> test structure with 4 atoms. (c) Comparison of the bandstructures computed with the HSE06 functional (red lines) and with DFT+ $J$  (black lines) with  $J = 40$  eV on Ge 4p and Si 3p orbitals for a 2H-Si<sub>1/2</sub>Ge<sub>1/2</sub> test structure with 4 atoms.

Fig. S2(b) compares the electronic band structure of a test Si<sub>1/4</sub>Ge<sub>3/4</sub> alloy cell computed using

the HSE06 hybrid functional and the DFT+ $J$  approach. The test structure consists of a four-atom cell in which one Ge atom is replaced by Si, corresponding to a 25% Si concentration. Matching the HSE06 bandgap of 0.62 eV requires a value of  $J = 40$  eV applied to the Ge 4*p* orbitals in the DFT+ $J$  formalism. This calibrated  $J$  value is then used for the larger alloy supercell and for the Si<sub>1/6</sub>Ge<sub>5/6</sub> alloy, as the local chemical environments of Ge atoms are sufficiently similar.

Fig. S2(c) compares the electronic band structure of a test Si<sub>1/2</sub>Ge<sub>1/2</sub> alloy cell computed using the HSE06 hybrid functional and the DFT+ $J$  approach. The test structure consists of a four-atom cell in which two Ge atoms are replaced by Si, corresponding to a 50% Si concentration. Matching the HSE06 direct bandgap requires applying  $J = 40$  eV to the Ge 4*p* and Si 3*p* orbitals in the DFT+ $J$  formalism.

Fig. S3(a) shows the absorption spectra of 2H-Ge computed with increasing densities of BZ sampling, including 80 bands and imposing a 2 Ry cutoff on the static screening matrix size. 2 valence and 2 conduction bands are considered. Spectra reach a reasonable convergence, in particular for the low-energy part, for  $21 \times 21 \times 14$   $k$ -point grids and denser.

Fig. S3(b) reports the absorption spectra of 2H-Ge computed on a  $9 \times 9 \times 6$   $k$ -point grid at varying static screening matrix size (2 Ry, 4 Ry and 6 Ry cutoffs) and number of included bands (60, 80, 100 and 200). 2 valence and 2 conduction bands are considered. Spectra vary minimally across all the sampled values.

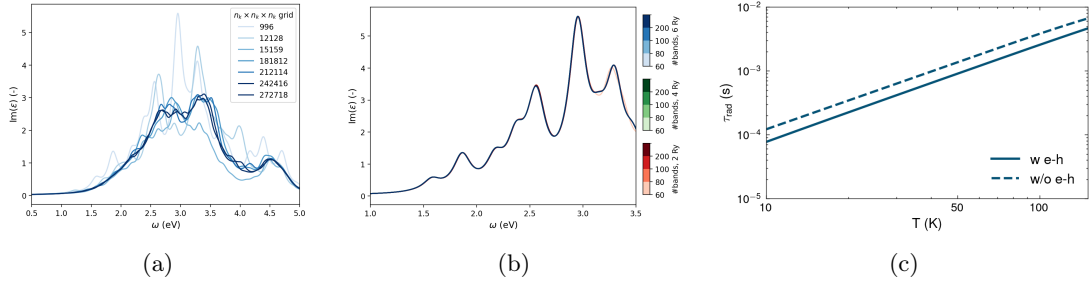

Figure S3: (a) Absorption spectra of 2H-Ge computed on different  $k$ -point grids. (b) Absorption spectra of 2H-Ge computed on a  $9 \times 9 \times 6$   $k$ -point grid for different sizes of the static screening matrix and number of included bands. (c) 2H-Ge radiative lifetime computed with the full BSE kernel (w e-h) and removing the exchange and direct electron-hole interactions in the BSE kernel (w/o e-h).

Fig. S3(c) shows the comparison between the radiative lifetime of 2H-Ge computed with the full BSE kernel (w e-h, solid line) and removing the exchange and direct electron-hole interactions (w/o e-h, dashed line) in the BSE kernel.
